# Supplementary material for: Two-component $GW$ calculations: Cubic scaling implementation and comparison of vertex corrected and partially self-consistent $GW$ variants
Source: arXiv:2303.09979 ancillary file (2023-05-17)
Supplement: Supplementary file 1 [file si.pdf]

# Supporting information to: Two-component $GW$ calculations: comparison of partially self-consistent variants and perturbative vertex corrections

Arno Förster,[*,†,‡] Erik van Lenthe,[*,†] Edoardo Spadetto,[†] and Lucas Visscher[‡]

†*Software for Chemistry and Materials NV, NL, 1081HV, Amsterdam, The Netherlands*

‡*Theoretical Chemistry, Vrije Universiteit, De Boelelaan 1083, NL-1081 HV, Amsterdam, The Netherlands*

E-mail: a.t.l.foerster@vu.nl; vanlenthe@scm.com

## A QP energies included in the benchmark

All QP energies calculated in this thesis are tabulated here. All values are in eV. The basis set limit extrapolation has been performed as stated in the main text. The 2C QP energies and the $G3W2$ corrected QP energies can be calculated form the values in the table by adding the terms $\Delta_{\text{SO}}$ and $\Delta_{G3W2}$, respectively.

The qs$GW$ calculations have only been calculated using ADF. To estimate the basis set limit, we have used the difference between the ADF and BAND extrapolated QP energies at the ev$GW$ level. This is considered as reliable, since the ev$GW$ results are very similar to the qs$GW$ ones.

Table 1: All $G_0W_0$@PBE QP energies calculated in this work for the systems included in the benchmark: ADF results (TZ3P, QZ6P, extrapolated), BAND results (TZ3P+, QZ6P+, extrapolated), spin-orbit correction, and $G3W2$ correction, both calculated using ADF with the QZ6P basis set. All values are in eV.

| Index | Name | ADF TZ3P | ADF QZ6P | ADF extra | BAND TZ3P+ | BAND QZ6P+ | BAND extra | $\Delta_{SO}$ | $\Delta_{G3W2}$ |
|---|---|---|---|---|---|---|---|---|---|
| 4 | $Al_2Br_6$ | 9.93 | 10.09 | 10.28 | 10.15 | 10.24 | 10.35 | −0.20 | 0.08 |
| 5 | $AlBr_3$ | 10.08 | 10.27 | 10.49 | 10.30 | 10.39 | 10.50 | −0.03 | 0.07 |
| 6 | $AlI_3$ | 9.02 | 9.00 | 8.96 | 9.14 | 9.17 | 9.23 | −0.10 | 0.06 |
| 7 | $AsBr_3$ | 9.33 | 9.48 | 9.66 | 9.58 | 9.65 | 9.74 | −0.02 | 0.03 |
| 8 | $AsCl_3$ | 9.97 | 10.27 | 10.60 | 10.09 | 10.24 | 10.46 | 0.00 | 0.00 |
| 9 | $AsF_3$ | 12.15 | 12.18 | 12.21 | 12.22 | 12.23 | 12.24 | 0.00 | 0.04 |
| 10 | $AsF_5$ | 14.27 | 14.27 | 14.28 | 14.29 | 14.32 | 14.36 | −0.01 | 0.22 |
| 11 | $AsH_3$ | 9.90 | 10.08 | 10.28 | 10.09 | 10.17 | 10.24 | 0.00 | −0.02 |
| 12 | $AsI_3$ | 8.64 | 8.65 | 8.67 | 8.77 | 8.90 | 9.11 | −0.16 | 0.08 |
| 13 | $Br_2$ | 9.90 | 10.06 | 10.24 | 10.15 | 10.26 | 10.38 | −0.14 | 0.06 |
| 14 | BrCl | 10.29 | 10.44 | 10.59 | 10.44 | 10.52 | 10.62 | −0.10 | 0.05 |
| 15 | $C_{10}H_{10}Ru$ | 6.45 | 6.53 | 6.63 | 6.59 | 6.73 | 6.90 | −0.01 | 0.01 |
| 16 | $C_2H_2Se$ | 8.09 | 8.22 | 8.37 | 8.21 | 8.28 | 8.35 | −0.01 | −0.04 |
| 17 | $C_2H_6Cd$ | 8.45 | 8.53 | 8.63 | 8.45 | 8.57 | 8.72 | 0.00 | −0.04 |
| 18 | $C_2H_6Hg$ | 8.64 | 8.73 | 8.84 | 8.61 | 8.80 | 9.03 | 0.02 | −0.06 |
| 19 | $C_2H_6Se$ | 7.76 | 7.93 | 8.12 | 7.95 | 8.06 | 8.19 | −0.01 | −0.03 |
| 20 | $C_2H_6Zn$ | 9.12 | 9.15 | 9.19 | 9.10 | 9.25 | 9.44 | 0.00 | −0.04 |
| 21 | $C_2HBrO$ | 8.66 | 8.79 | 8.94 | 8.74 | 8.86 | 8.99 | −0.01 | −0.05 |
| 22 | $C_4H_4Se$ | 8.32 | 8.48 | 8.67 | 8.34 | 8.53 | 8.75 | 0.00 | −0.08 |
| 23 | $CF_3I$ | 10.10 | 10.13 | 10.17 | 10.21 | 10.24 | 10.28 | −0.24 | 0.05 |
| 24 | $CH_3HgBr$ | 9.30 | 9.38 | 9.47 | 9.49 | 9.52 | 9.56 | −0.09 | 0.08 |
| 25 | $CH_3HgCl$ | 9.76 | 9.84 | 9.93 | 9.76 | 9.92 | 10.12 | 0.06 | 0.09 |
| 26 | $CH_3HgI$ | 8.68 | 8.68 | 8.68 | 8.78 | 8.76 | 8.72 | −0.18 | 0.06 |
| 27 | $CH_3I$ | 9.17 | 9.19 | 9.20 | 9.29 | 9.29 | 9.29 | −0.23 | 0.02 |
| 28 | $CI_4$ | 8.55 | 8.58 | 8.62 | 8.71 | 8.72 | 8.73 | −0.21 | 0.06 |
| 29 | $CaBr_2$ | 9.38 | 9.47 | 9.57 | 9.57 | 9.63 | 9.70 | −0.09 | 0.09 |
| 30 | $CaI_2$ | 8.74 | 8.75 | 8.77 | 8.83 | 8.86 | 8.92 | −0.19 | 0.07 |
| 31 | $CdBr_2$ | 9.76 | 9.90 | 10.08 | 9.97 | 10.03 | 10.12 | −0.10 | 0.11 |
| 32 | $CdCl_2$ | 10.34 | 10.55 | 10.78 | 10.36 | 10.50 | 10.73 | −0.03 | 0.11 |
| 33 | $CdI_2$ | 9.03 | 9.00 | 8.95 | 9.06 | 9.11 | 9.21 | −0.22 | 0.08 |
| 38 | $HgCl_2$ | 10.38 | 10.54 | 10.72 | 10.50 | 10.54 | 10.60 | −0.05 | 0.10 |
| 39 | $I_2$ | 8.96 | 8.98 | 9.02 | 9.11 | 9.24 | 9.48 | −0.27 | 0.05 |
| 40 | IBr | 9.33 | 9.42 | 9.55 | 9.54 | 9.57 | 9.61 | −0.24 | 0.05 |
| 41 | ICl | 9.63 | 9.70 | 9.80 | 9.72 | 9.79 | 9.92 | −0.24 | 0.05 |
| 42 | IF | 10.09 | 10.18 | 10.31 | 10.26 | 10.24 | 10.20 | −0.30 | 0.07 |
| 43 | KBr | 7.39 | 7.44 | 7.50 | 7.58 | 7.65 | 7.74 | −0.08 | 0.08 |
| 47 | $LaBr_3$ | 9.39 | 9.52 | 9.70 | 9.62 | 9.81 | 10.07 | −0.04 | 0.09 |
| 48 | $LaCl_3$ | 10.09 | 10.33 | 10.62 | 10.14 | 10.34 | 10.67 | −0.01 | 0.07 |
| 49 | LiBr | 8.52 | 8.61 | 8.70 | 8.74 | 8.77 | 8.82 | −0.09 | 0.10 |
| 50 | LiI | 7.98 | 7.96 | 7.93 | 8.08 | 8.11 | 8.16 | −0.18 | 0.07 |
| 51 | $MgBr_2$ | 10.04 | 10.11 | 10.21 | 10.24 | 10.32 | 10.42 | −0.08 | 0.10 |
| 52 | $MgI_2$ | 9.22 | 9.26 | 9.33 | 9.31 | 9.34 | 9.38 | −0.21 | 0.08 |
| 53 | $MoC_6O_6$ | 7.88 | 8.02 | 8.20 | 7.99 | 8.17 | 8.41 | −0.03 | −0.04 |
| 54 | NaBr | 7.87 | 7.88 | 7.89 | 8.04 | 7.97 | 7.88 | −0.10 | 0.09 |
| 55 | NaI | 7.44 | 7.40 | 7.34 | 7.53 | 7.57 | 7.64 | −0.16 | 0.08 |
| 56 | $OsO_4$ | 11.51 | 11.45 | 11.38 | 11.42 | 11.56 | 11.75 | 0.00 | 0.11 |
| 57 | $PBr_3$ | 9.17 | 9.27 | 9.38 | 9.34 | 9.41 | 9.51 | −0.01 | 0.00 |

Continued on next page

| Index | Name | ADF TZ3P | ADF QZ6P | ADF extra | BAND TZ3P+ | BAND QZ6P+ | BAND extra | $\Delta_{SO}$ | $\Delta_{G3W2}$ |
|---|---|---|---|---|---|---|---|---|---|
| 58 | $POBr_3$ | 10.19 | 10.38 | 10.59 | 10.35 | 10.48 | 10.63 | −0.09 | 0.09 |
| 62 | $RuO_4$ | 11.11 | 11.11 | 11.13 | 11.09 | 11.19 | 11.32 | 0.00 | 0.12 |
| 63 | $SOBr_2$ | 9.73 | 9.94 | 10.19 | 9.88 | 9.94 | 10.00 | −0.04 | 0.22 |
| 64 | $SPBr_3$ | 8.97 | 9.11 | 9.26 | 9.03 | 9.19 | 9.39 | −0.02 | 0.04 |
| 65 | $SeCl_2$ | 8.65 | 8.83 | 9.03 | 8.80 | 8.90 | 9.06 | −0.03 | 0.00 |
| 66 | $SeO_2$ | 11.01 | 10.87 | 10.70 | 10.97 | 10.93 | 10.88 | 0.00 | 0.10 |
| 67 | $SiBrF_3$ | 11.31 | 11.45 | 11.61 | 11.54 | 11.62 | 11.74 | −0.11 | 0.07 |
| 68 | $SiH_3I$ | 9.52 | 9.56 | 9.61 | 9.65 | 9.67 | 9.69 | −0.21 | 0.03 |
| 73 | $TiBr_4$ | 9.51 | 9.79 | 10.10 | 9.74 | 9.81 | 9.89 | −0.06 | 0.08 |
| 75 | $ZnBr_2$ | 10.08 | 10.30 | 10.55 | 10.29 | 10.37 | 10.47 | −0.13 | 0.09 |
| 79 | $ZrBr_4$ | 9.80 | 9.97 | 10.18 | 10.01 | 10.09 | 10.20 | −0.04 | 0.10 |
| 80 | $ZrCl_4$ | 10.74 | 10.97 | 11.23 | 10.75 | 10.90 | 11.14 | −0.01 | 0.10 |
| 81 | $ZrI_4$ | 8.75 | 8.80 | 8.89 | 8.87 | 8.98 | 9.19 | −0.15 | 0.07 |

Table 2: All $G_0W_0$@PBE0 QP energies calculated in this work for the systems included in the benchmark: ADF results (TZ3P, QZ6P, extrapolated), BAND results (TZ3P+, QZ6P+, extrapolated), spin-orbit correction, and $G3W2$ correction, both calculated using ADF with the QZ6P basis set. All values are in eV.

| Index | Name | ADF TZ3P | ADF QZ6P | ADF extra | BAND TZ3P+ | BAND QZ6P+ | BAND extra | $\Delta_{SO}$ | $\Delta_{G3W2}$ |
|---|---|---|---|---|---|---|---|---|---|
| 4 | $Al_2Br_6$ | 10.32 | 10.49 | 10.68 | 10.55 | 10.63 | 10.74 | −0.04 | 0.10 |
| 5 | $AlBr_3$ | 10.44 | 10.61 | 10.80 | 10.67 | 10.75 | 10.86 | −0.04 | 0.09 |
| 6 | $AlI_3$ | 9.35 | 9.38 | 9.44 | 9.51 | 9.52 | 9.55 | −0.15 | 0.06 |
| 7 | $AsBr_3$ | 9.64 | 9.85 | 10.09 | 9.90 | 10.00 | 10.13 | −0.08 | 0.03 |
| 8 | $AsCl_3$ | 10.32 | 10.57 | 10.83 | 10.43 | 10.59 | 10.81 | 0.00 | 0.00 |
| 9 | $AsF_3$ | 12.35 | 12.59 | 12.86 | 12.58 | 12.64 | 12.71 | 0.00 | 0.03 |
| 10 | $AsF_5$ | 15.00 | 15.11 | 15.22 | 15.01 | 15.14 | 15.31 | −0.01 | 0.26 |
| 11 | $AsH_3$ | 10.12 | 10.28 | 10.45 | 10.30 | 10.38 | 10.45 | 0.00 | −0.01 |
| 12 | $AsI_3$ | 8.90 | 9.04 | 9.27 | 9.08 | 9.13 | 9.20 | −0.26 | 0.10 |
| 13 | $Br_2$ | 10.14 | 10.30 | 10.48 | 10.40 | 10.49 | 10.60 | −0.15 | 0.07 |
| 14 | BrCl | 10.53 | 10.69 | 10.85 | 10.70 | 10.90 | 11.16 | −0.11 | 0.06 |
| 15 | $C_{10}H_{10}Ru$ | 6.67 | 6.76 | 6.87 | 6.88 | 7.02 | 7.20 | −0.08 | 0.06 |
| 16 | $C_2H_2Se$ | 8.31 | 8.46 | 8.64 | 8.45 | 8.57 | 8.72 | −0.01 | −0.04 |
| 17 | $C_2H_6Cd$ | 8.75 | 8.81 | 8.88 | 8.75 | 8.88 | 9.04 | 0.00 | −0.03 |
| 18 | $C_2H_6Hg$ | 8.88 | 8.95 | 9.02 | 8.78 | 9.05 | 9.35 | 0.03 | −0.05 |
| 19 | $C_2H_6Se$ | 7.96 | 8.13 | 8.32 | 8.16 | 8.23 | 8.31 | −0.01 | −0.02 |
| 20 | $C_2H_6Zn$ | 9.32 | 9.41 | 9.52 | 9.36 | 9.51 | 9.69 | 0.00 | −0.03 |
| 21 | $C_2HBrO$ | 8.95 | 9.11 | 9.29 | 9.04 | 9.18 | 9.35 | −0.01 | −0.06 |
| 22 | $C_4H_4Se$ | 8.47 | 8.73 | 9.03 | 8.62 | 8.81 | 9.03 | 0.00 | −0.07 |
| 23 | $CF_3I$ | 10.40 | 10.43 | 10.46 | 10.54 | 10.56 | 10.58 | −0.27 | 0.06 |
| 24 | $CH_3HgBr$ | 9.64 | 9.73 | 9.84 | 9.83 | 9.91 | 10.00 | −0.11 | 0.11 |
| 25 | $CH_3HgCl$ | 10.18 | 10.35 | 10.55 | 10.17 | 10.38 | 10.63 | −0.03 | 0.11 |
| 26 | $CH_3HgI$ | 8.96 | 8.99 | 9.04 | 9.08 | 9.08 | 9.07 | −0.23 | 0.08 |
| 27 | $CH_3I$ | 9.37 | 9.40 | 9.45 | 9.50 | 9.55 | 9.61 | −0.26 | 0.03 |
| 28 | $CI_4$ | 8.86 | 8.90 | 8.97 | 9.02 | 9.07 | 9.15 | −0.21 | 0.07 |
| 29 | $CaBr_2$ | 9.75 | 9.90 | 10.07 | 9.96 | 10.00 | 10.05 | −0.11 | 0.12 |
| 30 | $CaI_2$ | 9.06 | 9.09 | 9.15 | 9.19 | 9.17 | 9.13 | −0.23 | 0.10 |
| 31 | $CdBr_2$ | 10.14 | 10.27 | 10.43 | 10.33 | 10.40 | 10.48 | −0.13 | 0.13 |
| 32 | $CdCl_2$ | 10.80 | 10.96 | 11.15 | 10.81 | 10.97 | 11.22 | −0.03 | 0.14 |

Continued on next page

| Index | Name | ADF TZ3P | ADF QZ6P | ADF extra | BAND TZ3P+ | BAND QZ6P+ | BAND extra | $\Delta_{SO}$ | $\Delta_{G3W2}$ |
|---|---|---|---|---|---|---|---|---|---|
| 33 | $CdI_2$ | 9.33 | 9.35 | 9.39 | 9.46 | 9.47 | 9.49 | −0.26 | 0.10 |
| 38 | $HgCl_2$ | 10.77 | 10.94 | 11.14 | 10.89 | 10.96 | 11.06 | −0.06 | 0.12 |
| 39 | $I_2$ | 9.18 | 9.22 | 9.30 | 9.35 | 9.42 | 9.53 | −0.30 | 0.05 |
| 40 | IBr | 9.60 | 9.69 | 9.82 | 9.80 | 9.79 | 9.78 | −0.27 | 0.06 |
| 41 | ICl | 9.87 | 9.92 | 9.98 | 9.99 | 10.05 | 10.13 | −0.27 | 0.05 |
| 42 | IF | 10.37 | 10.42 | 10.48 | 10.50 | 10.54 | 10.60 | −0.31 | 0.07 |
| 43 | KBr | 7.71 | 7.83 | 7.98 | 7.91 | 7.97 | 8.05 | −0.11 | 0.11 |
| 47 | $LaBr_3$ | 9.88 | 10.04 | 10.23 | 10.10 | 10.11 | 10.13 | −0.07 | 0.14 |
| 48 | $LaCl_3$ | 10.62 | 10.79 | 10.99 | 10.64 | 10.83 | 11.15 | −0.01 | 0.12 |
| 49 | LiBr | 8.81 | 8.92 | 9.03 | 9.02 | 9.07 | 9.12 | −0.10 | 0.12 |
| 50 | LiI | 8.22 | 8.25 | 8.28 | 8.35 | 8.33 | 8.30 | −0.22 | 0.09 |
| 51 | $MgBr_2$ | 10.41 | 10.55 | 10.73 | 10.62 | 10.69 | 10.78 | −0.12 | 0.12 |
| 52 | $MgI_2$ | 9.47 | 9.57 | 9.77 | 9.67 | 9.69 | 9.74 | −0.25 | 0.09 |
| 53 | $MoC_6O_6$ | 8.16 | 8.30 | 8.49 | 8.28 | 8.46 | 8.72 | −0.04 | −0.03 |
| 54 | NaBr | 8.16 | 8.28 | 8.42 | 8.37 | 8.40 | 8.45 | −0.11 | 0.12 |
| 55 | NaI | 7.72 | 7.74 | 7.79 | 7.83 | 7.80 | 7.75 | −0.22 | 0.10 |
| 56 | $OsO_4$ | 12.05 | 12.04 | 12.01 | 11.98 | 12.13 | 12.33 | −0.01 | 0.20 |
| 57 | $PBr_3$ | 9.49 | 9.64 | 9.81 | 9.66 | 9.75 | 9.87 | −0.03 | 0.00 |
| 58 | $POBr_3$ | 10.64 | 10.81 | 10.99 | 10.89 | 10.95 | 11.02 | −0.12 | 0.10 |
| 62 | $RuO_4$ | 11.85 | 11.88 | 11.92 | 11.85 | 11.91 | 12.00 | 0.00 | 0.25 |
| 63 | $SOBr_2$ | 10.13 | 10.31 | 10.52 | 10.27 | 10.41 | 10.59 | −0.05 | 0.04 |
| 64 | $SPBr_3$ | 9.31 | 9.48 | 9.67 | 9.37 | 9.54 | 9.77 | −0.02 | 0.06 |
| 65 | $SeCl_2$ | 8.94 | 9.15 | 9.39 | 9.10 | 9.25 | 9.45 | −0.02 | 0.00 |
| 66 | $SeO_2$ | 11.39 | 11.40 | 11.42 | 11.43 | 11.51 | 11.61 | −0.01 | 0.13 |
| 67 | $SiBrF_3$ | 11.62 | 11.77 | 11.94 | 11.84 | 11.88 | 11.94 | −0.13 | 0.08 |
| 68 | $SiH_3I$ | 9.76 | 9.80 | 9.86 | 9.91 | 9.92 | 9.95 | −0.25 | 0.04 |
| 73 | $TiBr_4$ | 10.08 | 10.26 | 10.47 | 10.30 | 10.42 | 10.56 | −0.09 | 0.15 |
| 75 | $ZnBr_2$ | 10.43 | 10.57 | 10.75 | 10.65 | 10.75 | 10.87 | −0.13 | 0.11 |
| 79 | $ZrBr_4$ | 10.29 | 10.46 | 10.68 | 10.50 | 10.63 | 10.80 | −0.09 | 0.13 |
| 80 | $ZrCl_4$ | 11.32 | 11.50 | 11.72 | 11.32 | 11.47 | 11.72 | −0.02 | 0.14 |
| 81 | $ZrI_4$ | 9.16 | 9.21 | 9.30 | 9.31 | 9.36 | 9.44 | −0.19 | 0.10 |

Table 3: All $G_0W_0$@BHLYP QP energies calculated in this work for the systems included in the benchmark: ADF results (TZ3P, QZ6P, extrapolated), BAND results (TZ3P+, QZ6P+, extrapolated), spin-orbit correction, and $G3W2$ correction, both calculated using ADF with the QZ6P basis set. All values are in eV.

| Index | Name | ADF TZ3P | ADF QZ6P | ADF extra | BAND TZ3P+ | BAND QZ6P+ | BAND extra | $\Delta_{SO}$ | $\Delta_{G3W2}$ |
|---|---|---|---|---|---|---|---|---|---|
| 4 | $Al_2Br_6$ | 10.61 | 10.78 | 10.97 | 10.84 | 10.91 | 11.00 | −0.04 | 0.10 |
| 5 | $AlBr_3$ | 10.69 | 10.86 | 11.06 | 10.93 | 10.99 | 11.07 | −0.04 | 0.10 |
| 6 | $AlI_3$ | 9.61 | 9.65 | 9.71 | 9.77 | 9.79 | 9.82 | −0.17 | 0.07 |
| 7 | $AsBr_3$ | 9.90 | 10.11 | 10.36 | 10.17 | 10.23 | 10.30 | −0.06 | 0.03 |
| 8 | $AsCl_3$ | 10.60 | 10.85 | 11.11 | 10.72 | 10.89 | 11.12 | −0.01 | 0.00 |
| 9 | $AsF_3$ | 12.70 | 12.93 | 13.19 | 12.88 | 12.98 | 13.11 | 0.00 | 0.03 |
| 10 | $AsF_5$ | 15.48 | 15.61 | 15.74 | 15.47 | 15.62 | 15.80 | −0.01 | 0.30 |
| 11 | $AsH_3$ | 10.29 | 10.50 | 10.72 | 10.47 | 10.56 | 10.64 | 0.00 | −0.01 |
| 12 | $AsI_3$ | 9.16 | 9.20 | 9.28 | 9.34 | 9.39 | 9.46 | −0.19 | 0.04 |
| 13 | $Br_2$ | 10.34 | 10.51 | 10.70 | 10.59 | 10.62 | 10.66 | −0.17 | 0.07 |
| 14 | BrCl | 10.74 | 10.93 | 11.13 | 10.89 | 11.01 | 11.18 | −0.12 | 0.07 |

Continued on next page

| Index | Name | ADF TZ3P | ADF QZ6P | ADF extra | BAND TZ3P+ | BAND QZ6P+ | BAND extra | $\Delta_{SO}$ | $\Delta_{G3W2}$ |
|---|---|---|---|---|---|---|---|---|---|
| 15 | $C_{10}H_{10}Ru$ | 7.00 | 7.10 | 7.23 | 7.22 | 7.36 | 7.54 | −0.11 | 0.10 |
| 16 | $C_2H_2Se$ | 8.47 | 8.63 | 8.83 | 8.61 | 8.73 | 8.88 | −0.01 | −0.04 |
| 17 | $C_2H_6Cd$ | 8.92 | 9.01 | 9.11 | 8.92 | 9.10 | 9.32 | 0.00 | −0.02 |
| 18 | $C_2H_6Hg$ | 9.03 | 9.13 | 9.25 | 8.96 | 9.26 | 9.60 | 0.05 | −0.04 |
| 19 | $C_2H_6Se$ | 8.13 | 8.32 | 8.53 | 8.34 | 8.43 | 8.53 | 0.00 | −0.02 |
| 20 | $C_2H_6Zn$ | 9.50 | 9.61 | 9.73 | 9.51 | 9.69 | 9.90 | 0.00 | −0.02 |
| 21 | $C_2HBrO$ | 9.19 | 9.33 | 9.51 | 9.27 | 9.43 | 9.62 | −0.01 | −0.06 |
| 22 | $C_4H_4Se$ | 8.83 | 8.93 | 9.05 | 8.81 | 8.98 | 9.19 | 0.00 | −0.07 |
| 23 | $CF_3I$ | 10.69 | 10.73 | 10.77 | 10.85 | 10.86 | 10.88 | −0.30 | 0.07 |
| 24 | $CH_3HgBr$ | 9.85 | 9.97 | 10.12 | 10.07 | 10.13 | 10.21 | −0.13 | 0.13 |
| 25 | $CH_3HgCl$ | 10.45 | 10.62 | 10.82 | 10.42 | 10.61 | 10.85 | −0.03 | 0.14 |
| 26 | $CH_3HgI$ | 9.17 | 9.22 | 9.28 | 9.29 | 9.30 | 9.30 | −0.25 | 0.10 |
| 27 | $CH_3I$ | 9.54 | 9.59 | 9.66 | 9.69 | 9.71 | 9.75 | −0.29 | 0.04 |
| 28 | $CI_4$ | 9.13 | 9.18 | 9.26 | 9.30 | 9.35 | 9.45 | −0.22 | 0.08 |
| 29 | $CaBr_2$ | 9.98 | 10.13 | 10.30 | 10.19 | 10.25 | 10.33 | −0.14 | 0.15 |
| 30 | $CaI_2$ | 9.28 | 9.33 | 9.42 | 9.42 | 9.41 | 9.37 | −0.27 | 0.12 |
| 31 | $CdBr_2$ | 10.39 | 10.51 | 10.66 | 10.59 | 10.65 | 10.74 | −0.14 | 0.15 |
| 32 | $CdCl_2$ | 11.08 | 11.28 | 11.50 | 11.09 | 11.22 | 11.43 | −0.04 | 0.16 |
| 33 | $CdI_2$ | 9.56 | 9.60 | 9.66 | 9.71 | 9.73 | 9.76 | −0.29 | 0.11 |
| 38 | $HgCl_2$ | 11.04 | 11.22 | 11.43 | 11.14 | 11.21 | 11.32 | −0.06 | 0.14 |
| 39 | $I_2$ | 9.38 | 9.42 | 9.49 | 9.54 | 9.62 | 9.76 | −0.33 | 0.06 |
| 40 | IBr | 9.78 | 9.87 | 10.00 | 9.97 | 10.01 | 10.07 | −0.28 | 0.06 |
| 41 | ICl | 10.08 | 10.15 | 10.26 | 10.19 | 10.27 | 10.42 | −0.28 | 0.06 |
| 42 | IF | 10.60 | 10.64 | 10.72 | 10.73 | 10.78 | 10.85 | −0.32 | 0.07 |
| 43 | KBr | 7.89 | 8.04 | 8.20 | 8.11 | 8.16 | 8.24 | −0.13 | 0.13 |
| 47 | $LaBr_3$ | 10.19 | 10.34 | 10.52 | 10.41 | 10.48 | 10.58 | −0.09 | 0.18 |
| 48 | $LaCl_3$ | 10.97 | 11.14 | 11.35 | 10.98 | 11.19 | 11.55 | −0.01 | 0.15 |
| 49 | LiBr | 9.00 | 9.15 | 9.31 | 9.21 | 9.27 | 9.34 | −0.13 | 0.13 |
| 50 | LiI | 8.40 | 8.43 | 8.48 | 8.53 | 8.54 | 8.56 | −0.26 | 0.10 |
| 51 | $MgBr_2$ | 10.63 | 10.79 | 10.98 | 10.85 | 10.89 | 10.95 | −0.14 | 0.14 |
| 52 | $MgI_2$ | 9.75 | 9.80 | 9.90 | 9.90 | 9.92 | 9.96 | −0.28 | 0.10 |
| 53 | $MoC_6O_6$ | 8.47 | 8.61 | 8.80 | 8.60 | 8.77 | 9.01 | −0.02 | −0.01 |
| 54 | NaBr | 8.37 | 8.51 | 8.67 | 8.58 | 8.62 | 8.67 | −0.13 | 0.14 |
| 55 | NaI | 7.91 | 7.94 | 7.98 | 8.03 | 8.03 | 8.03 | −0.25 | 0.11 |
| 56 | $OsO_4$ | 12.52 | 12.53 | 12.53 | 12.49 | 12.61 | 12.78 | −0.06 | 0.30 |
| 57 | $PBr_3$ | 9.78 | 9.91 | 10.06 | 9.93 | 9.99 | 10.06 | −0.03 | 0.00 |
| 58 | $POBr_3$ | 10.97 | 11.14 | 11.33 | 11.21 | 11.26 | 11.33 | −0.13 | 0.11 |
| 62 | $RuO_4$ | 12.30 | 12.37 | 12.45 | 12.31 | 12.41 | 12.56 | −0.01 | 0.41 |
| 63 | $SOBr_2$ | 10.44 | 10.59 | 10.76 | 10.57 | 10.68 | 10.82 | −0.06 | 0.05 |
| 64 | $SPBr_3$ | 9.56 | 9.72 | 9.90 | 9.62 | 9.78 | 9.98 | −0.02 | 0.08 |
| 65 | $SeCl_2$ | 9.19 | 9.39 | 9.62 | 9.35 | 9.48 | 9.66 | −0.01 | 0.01 |
| 66 | $SeO_2$ | 11.64 | 11.74 | 11.86 | 11.38 | 11.81 | 12.35 | 0.00 | 0.16 |
| 67 | $SiBrF_3$ | 11.86 | 12.01 | 12.17 | 12.09 | 12.13 | 12.19 | −0.14 | 0.09 |
| 68 | $SiH_3I$ | 9.96 | 10.01 | 10.07 | 10.10 | 10.13 | 10.16 | −0.27 | 0.05 |
| 73 | $TiBr_4$ | 10.46 | 10.63 | 10.83 | 10.69 | 10.77 | 10.87 | −0.10 | 0.22 |
| 75 | $ZnBr_2$ | 10.66 | 10.81 | 10.99 | 10.88 | 10.93 | 10.99 | −0.15 | 0.13 |
| 79 | $ZrBr_4$ | 10.64 | 10.81 | 11.01 | 10.85 | 10.92 | 11.02 | −0.10 | 0.17 |
| 80 | $ZrCl_4$ | 11.72 | 11.89 | 12.08 | 11.72 | 11.89 | 12.15 | −0.02 | 0.18 |
| 81 | $ZrI_4$ | 9.49 | 9.55 | 9.65 | 9.65 | 9.70 | 9.78 | −0.22 | 0.13 |

Table 4: All ev$GW$@PBE0 QP energies calculated in this work for the systems included in the benchmark: ADF results (TZ3P, QZ6P, extrapolated), BAND results (TZ3P+, QZ6P+, extrapolated), spin-orbit correction, and $G3W2$ correction, both calculated using ADF with the QZ6P basis set. All values are in eV.

| | | ADF | | | BAND | | | | |
|---|---|---|---|---|---|---|---|---|---|
| Index | Name | TZ3P | QZ6P | extra | TZ3P+ | QZ6P+ | extra | $\Delta_{SO}$ | $\Delta_{G3W2}$ |
| 4 | $Al_2Br_6$ | 10.65 | 10.85 | 11.08 | 10.93 | 11.01 | 11.10 | −0.04 | 0.11 |
| 5 | $AlBr_3$ | 10.77 | 10.96 | 11.19 | 11.04 | 11.11 | 11.20 | −0.04 | 0.11 |
| 6 | $AlI_3$ | 9.64 | 9.68 | 9.75 | 9.76 | 9.85 | 9.99 | −0.16 | 0.08 |
| 7 | $AsBr_3$ | 9.90 | 10.13 | 10.39 | 10.19 | 10.29 | 10.42 | −0.04 | 0.03 |
| 8 | $AsCl_3$ | 10.58 | 10.86 | 11.16 | 10.70 | 10.90 | 11.17 | 0.00 | 0.00 |
| 9 | $AsF_3$ | 12.73 | 12.98 | 13.25 | 12.90 | 13.03 | 13.19 | 0.00 | 0.04 |
| 10 | $AsF_5$ | 15.74 | 15.90 | 16.07 | 15.75 | 15.93 | 16.15 | −0.01 | 0.34 |
| 11 | $AsH_3$ | 10.34 | 10.55 | 10.78 | 10.53 | 10.65 | 10.77 | 0.00 | −0.01 |
| 12 | $AsI_3$ | 9.14 | 9.35 | 9.70 | 9.34 | 9.40 | 9.49 | −0.31 | 0.13 |
| 13 | $Br_2$ | 10.41 | 10.60 | 10.82 | 10.69 | 10.77 | 10.85 | −0.16 | 0.08 |
| 14 | BrCl | 10.81 | 11.03 | 11.26 | 10.98 | 11.12 | 11.30 | −0.12 | 0.07 |
| 15 | $C_{10}H_{10}Ru$ | 6.90 | 7.02 | 7.16 | 7.14 | 7.31 | 7.52 | −0.08 | 0.10 |
| 16 | $C_2H_2Se$ | 8.49 | 8.67 | 8.88 | 8.63 | 8.77 | 8.95 | −0.01 | −0.04 |
| 17 | $C_2H_6Cd$ | 9.00 | 9.11 | 9.24 | 9.02 | 9.21 | 9.45 | 0.00 | −0.01 |
| 18 | $C_2H_6Hg$ | 9.08 | 9.20 | 9.34 | 9.02 | 9.31 | 9.64 | 0.03 | −0.04 |
| 19 | $C_2H_6Se$ | 8.20 | 8.39 | 8.60 | 8.41 | 8.51 | 8.63 | −0.01 | −0.02 |
| 20 | $C_2H_6Zn$ | 9.61 | 9.74 | 9.88 | 9.66 | 9.84 | 10.05 | 0.00 | −0.01 |
| 21 | $C_2HBrO$ | 9.16 | 9.33 | 9.53 | 9.26 | 9.42 | 9.62 | −0.01 | −0.06 |
| 22 | $C_4H_4Se$ | 8.80 | 8.94 | 9.10 | 8.82 | 9.02 | 9.26 | 0.01 | −0.07 |
| 23 | $CF_3I$ | 10.64 | 10.68 | 10.73 | 10.80 | 10.82 | 10.85 | −0.29 | 0.07 |
| 24 | $CH_3HgBr$ | 9.97 | 10.13 | 10.32 | 10.20 | 10.31 | 10.44 | −0.12 | 0.14 |
| 25 | $CH_3HgCl$ | 10.61 | 10.80 | 11.02 | 10.57 | 10.84 | 11.17 | −0.03 | 0.15 |
| 26 | $CH_3HgI$ | 9.26 | 9.29 | 9.34 | 9.38 | 9.43 | 9.51 | −0.25 | 0.10 |
| 27 | $CH_3I$ | 9.60 | 9.64 | 9.70 | 9.75 | 9.78 | 9.82 | −0.28 | 0.04 |
| 28 | $CI_4$ | 9.12 | 9.15 | 9.21 | 9.30 | 9.36 | 9.46 | −0.22 | 0.08 |
| 29 | $CaBr_2$ | 10.10 | 10.27 | 10.47 | 10.34 | 10.41 | 10.49 | −0.13 | 0.16 |
| 30 | $CaI_2$ | 9.35 | 9.41 | 9.50 | 9.51 | 9.52 | 9.53 | −0.27 | 0.12 |
| 31 | $CdBr_2$ | 10.50 | 10.68 | 10.89 | 10.75 | 10.79 | 10.85 | −0.14 | 0.16 |
| 32 | $CdCl_2$ | 11.25 | 11.44 | 11.67 | 11.26 | 11.45 | 11.76 | −0.04 | 0.18 |
| 33 | $CdI_2$ | 9.65 | 9.68 | 9.72 | 9.79 | 9.83 | 9.92 | −0.29 | 0.12 |
| 38 | $HgCl_2$ | 11.19 | 11.38 | 11.59 | 11.29 | 11.40 | 11.55 | −0.07 | 0.16 |
| 39 | $I_2$ | 9.41 | 9.45 | 9.53 | 9.58 | 9.67 | 9.81 | −0.32 | 0.06 |
| 40 | IBr | 9.81 | 9.92 | 10.08 | 10.03 | 10.07 | 10.13 | −0.28 | 0.07 |
| 41 | ICl | 10.10 | 10.20 | 10.35 | 10.25 | 10.30 | 10.37 | −0.29 | 0.06 |
| 42 | IF | 10.61 | 10.66 | 10.74 | 10.76 | 10.80 | 10.86 | −0.34 | 0.07 |
| 43 | KBr | 8.07 | 8.24 | 8.45 | 8.31 | 8.40 | 8.53 | −0.12 | 0.14 |
| 47 | $LaBr_3$ | 10.30 | 10.47 | 10.69 | 10.55 | 10.61 | 10.70 | −0.09 | 0.18 |
| 48 | $LaCl_3$ | 11.05 | 11.26 | 11.50 | 11.08 | 11.30 | 11.67 | −0.01 | 0.16 |
| 49 | LiBr | 9.16 | 9.32 | 9.50 | 9.40 | 9.47 | 9.55 | −0.12 | 0.15 |
| 50 | LiI | 8.51 | 8.55 | 8.61 | 8.64 | 8.67 | 8.71 | −0.25 | 0.12 |
| 51 | $MgBr_2$ | 10.77 | 10.94 | 11.16 | 11.01 | 11.08 | 11.17 | −0.13 | 0.15 |
| 52 | $MgI_2$ | 9.85 | 9.88 | 9.95 | 9.99 | 10.04 | 10.12 | −0.28 | 0.11 |
| 53 | $MoC_6O_6$ | 8.31 | 8.47 | 8.70 | 8.44 | 8.64 | 8.92 | −0.05 | −0.02 |
| 54 | NaBr | 8.54 | 8.71 | 8.91 | 8.78 | 8.87 | 8.98 | −0.13 | 0.15 |
| 55 | NaI | 8.04 | 8.07 | 8.12 | 8.17 | 8.19 | 8.23 | −0.25 | 0.12 |
| 56 | $OsO_4$ | 12.60 | 12.65 | 12.72 | 12.56 | 12.73 | 12.95 | −0.02 | 0.35 |
| 57 | $PBr_3$ | 9.74 | 9.90 | 10.09 | 9.92 | 10.04 | 10.18 | −0.03 | 0.00 |

Continued on next page

| Index | Name | ADF TZ3P | ADF QZ6P | ADF extra | BAND TZ3P+ | BAND QZ6P+ | BAND extra | $\Delta_{SO}$ | $\Delta_{G3W2}$ |
|---|---|---|---|---|---|---|---|---|---|
| 58 | $POBr_3$ | 10.97 | 11.15 | 11.36 | 11.24 | 11.30 | 11.38 | −0.11 | 0.12 |
| 62 | $RuO_4$ | 12.35 | 12.50 | 12.71 | 12.41 | 12.49 | 12.60 | 0.00 | 0.47 |
| 63 | $SOBr_2$ | 10.45 | 10.61 | 10.80 | 10.61 | 10.74 | 10.91 | −0.03 | 0.06 |
| 64 | $SPBr_3$ | 9.62 | 9.79 | 9.99 | 9.70 | 9.88 | 10.10 | −0.02 | 0.09 |
| 65 | $SeCl_2$ | 9.19 | 9.41 | 9.67 | 9.36 | 9.51 | 9.72 | −0.02 | 0.01 |
| 66 | $SeO_2$ | 11.80 | 11.89 | 12.01 | 11.86 | 11.97 | 12.10 | −0.01 | 0.20 |
| 67 | $SiBrF_3$ | 11.91 | 12.07 | 12.25 | 12.15 | 12.21 | 12.30 | −0.13 | 0.10 |
| 68 | $SiH_3I$ | 10.02 | 10.07 | 10.13 | 10.17 | 10.21 | 10.27 | −0.27 | 0.05 |
| 73 | $TiBr_4$ | 10.49 | 10.69 | 10.91 | 10.77 | 10.85 | 10.95 | −0.09 | 0.21 |
| 75 | $ZnBr_2$ | 10.78 | 10.97 | 11.19 | 11.04 | 11.10 | 11.17 | −0.14 | 0.14 |
| 79 | $ZrBr_4$ | 10.69 | 10.88 | 11.12 | 10.97 | 11.03 | 11.10 | −0.09 | 0.18 |
| 80 | $ZrCl_4$ | 11.78 | 11.99 | 12.22 | 11.79 | 12.00 | 12.33 | −0.02 | 0.19 |
| 81 | $ZrI_4$ | 9.50 | 9.54 | 9.61 | 9.67 | 9.72 | 9.83 | −0.21 | 0.14 |

Table 5: All qs*GW* QP energies calculated calculated in this work for the systems included in the benchmark: ADF results (TZ3P, QZ6P, extrapolated), correction due to difference of ev*GW* QP energies calculated with ADF and BAND, final, corrected qs*GW* QP energies, spin-orbit correction, and $G3W2$ correction (the latter two calculated using ADF with the QZ6P basis set). All values are in eV.

| Index | Name | ADF TZ3P | ADF QZ6P | ADF extra | $\Delta_{evGW}$ | extra | $\Delta_{SO}$ | $\Delta_{G3W2}$ |
|---|---|---|---|---|---|---|---|---|
| 4 | $Al_2Br_6$ | 10.94 | 10.94 | 10.94 | 0.01 | 10.95 | −0.04 | 0.14 |
| 5 | $AlBr_3$ | 11.04 | 11.07 | 11.12 | 0.02 | 11.14 | −0.06 | 0.10 |
| 6 | $AlI_3$ | 9.82 | 9.85 | 9.91 | 0.23 | 10.15 | −0.17 | 0.08 |
| 7 | $AsBr_3$ | 10.18 | 10.25 | 10.33 | 0.03 | 10.35 | −0.03 | 0.02 |
| 8 | $AsCl_3$ | 10.82 | 10.97 | 11.14 | 0.01 | 11.15 | 0.00 | −0.01 |
| 9 | $AsF_3$ | 13.11 | 13.19 | 13.27 | −0.06 | 13.21 | 0.02 | 0.02 |
| 10 | $AsF_5$ | 16.09 | 16.07 | 16.05 | 0.09 | 16.14 | −0.01 | 0.44 |
| 11 | $AsH_3$ | 10.55 | 10.64 | 10.74 | −0.02 | 10.72 | 0.00 | −0.02 |
| 12 | $AsI_3$ | 9.32 | 9.38 | 9.48 | −0.21 | 9.28 | −0.23 | 0.04 |
| 13 | $Br_2$ | 10.64 | 10.69 | 10.74 | 0.03 | 10.77 | −0.20 | 0.08 |
| 14 | BrCl | 11.01 | 11.10 | 11.18 | 0.04 | 11.23 | −0.12 | 0.07 |
| 15 | $C_{10}H_{10}Ru$ | 7.33 | 7.43 | 7.57 | 0.36 | 7.93 | −0.13 | 0.10 |
| 16 | $C_2H_2Se$ | 8.62 | 8.73 | 8.86 | 0.07 | 8.94 | 0.02 | −0.04 |
| 17 | $C_2H_6Cd$ | 9.06 | 9.14 | 9.25 | 0.22 | 9.46 | 0.01 | −0.01 |
| 18 | $C_2H_6Hg$ | 9.18 | 9.26 | 9.37 | 0.30 | 9.67 | 0.07 | −0.04 |
| 19 | $C_2H_6Se$ | 8.42 | 8.49 | 8.58 | 0.04 | 8.61 | 0.00 | −0.01 |
| 20 | $C_2H_6Zn$ | 9.68 | 9.75 | 9.84 | 0.17 | 10.01 | 0.00 | −0.01 |
| 21 | $C_2HBrO$ | 9.31 | 9.40 | 9.52 | 0.09 | 9.61 | −0.01 | −0.06 |
| 22 | $C_4H_4Se$ | 8.84 | 8.91 | 8.99 | 0.16 | 9.15 | 0.04 | −0.03 |
| 23 | $CF_3I$ | 10.91 | 10.93 | 10.95 | 0.12 | 11.07 | −0.33 | 0.07 |
| 24 | $CH_3HgBr$ | 10.22 | 10.26 | 10.30 | 0.12 | 10.43 | −0.09 | 0.14 |
| 25 | $CH_3HgCl$ | 10.77 | 10.86 | 10.95 | 0.15 | 11.10 | 0.00 | 0.15 |
| 26 | $CH_3HgI$ | 9.40 | 9.45 | 9.51 | 0.16 | 9.67 | −0.27 | 0.10 |
| 27 | $CH_3I$ | 9.75 | 9.79 | 9.84 | 0.12 | 9.96 | −0.33 | 0.05 |
| 28 | $CI_4$ | 9.31 | 9.34 | 9.39 | 0.25 | 9.63 | −0.23 | 0.08 |
| 29 | $CaBr_2$ | 10.33 | 10.35 | 10.38 | 0.02 | 10.40 | −0.17 | 0.16 |
| 30 | $CaI_2$ | 9.50 | 9.55 | 9.65 | 0.03 | 9.68 | −0.33 | 0.12 |

Continued on next page

| Index | Name | ADF TZ3P | QZ6P | extra | $\Delta_{evGW}$ | extra | $\Delta_{SO}$ | $\Delta_{G3W2}$ |
|---|---|---|---|---|---|---|---|---|
| 31 | $CdBr_2$ | 10.75 | 10.76 | 10.78 | −0.04 | 10.74 | −0.17 | 0.16 |
| 32 | $CdCl_2$ | 11.38 | 11.46 | 11.55 | 0.09 | 11.64 | 0.00 | 0.17 |
| 33 | $CdI_2$ | 9.79 | 9.83 | 9.89 | 0.19 | 10.09 | −0.32 | 0.12 |
| 38 | $HgCl_2$ | 11.34 | 11.42 | 11.51 | −0.04 | 11.47 | −0.05 | 0.15 |
| 39 | $I_2$ | 9.56 | 9.59 | 9.64 | 0.28 | 9.92 | −0.38 | 0.06 |
| 40 | IBr | 10.02 | 10.05 | 10.11 | 0.06 | 10.17 | −0.33 | 0.07 |
| 41 | ICl | 10.28 | 10.32 | 10.38 | 0.03 | 10.40 | −0.20 | 0.06 |
| 42 | IF | 10.82 | 10.84 | 10.85 | 0.12 | 10.98 | −0.33 | 0.07 |
| 43 | KBr | 8.25 | 8.27 | 8.30 | 0.08 | 8.38 | −0.17 | 0.14 |
| 47 | $LaBr_3$ | 10.55 | 10.59 | 10.63 | 0.01 | 10.64 | −0.13 | 0.19 |
| 48 | $LaCl_3$ | 11.24 | 11.36 | 11.51 | 0.17 | 11.68 | −0.01 | 0.17 |
| 49 | LiBr | 9.34 | 9.37 | 9.40 | 0.05 | 9.45 | −0.16 | 0.14 |
| 50 | LiI | 8.58 | 8.64 | 8.73 | 0.10 | 8.83 | −0.24 | 0.11 |
| 51 | $MgBr_2$ | 10.98 | 11.01 | 11.04 | 0.01 | 11.05 | −0.17 | 0.15 |
| 52 | $MgI_2$ | 9.96 | 10.03 | 10.15 | 0.17 | 10.31 | −0.35 | 0.11 |
| 53 | $MoC_6O_6$ | 8.50 | 8.65 | 8.85 | 0.23 | 9.08 | −0.09 | −0.01 |
| 54 | NaBr | 8.71 | 8.74 | 8.77 | 0.07 | 8.83 | −0.16 | 0.14 |
| 55 | NaI | 8.09 | 8.14 | 8.23 | 0.10 | 8.33 | −0.32 | 0.12 |
| 56 | $OsO_4$ | 12.75 | 12.74 | 12.73 | 0.23 | 12.96 | −0.25 | 0.37 |
| 57 | $PBr_3$ | 9.99 | 10.01 | 10.03 | 0.09 | 10.12 | −0.04 | −0.01 |
| 58 | $POBr_3$ | 11.28 | 11.31 | 11.35 | 0.02 | 11.37 | −0.10 | 0.12 |
| 62 | $RuO_4$ | 12.56 | 12.54 | 12.52 | −0.11 | 12.41 | −0.06 | 0.51 |
| 63 | $SOBr_2$ | 10.68 | 10.74 | 10.81 | 0.11 | 10.92 | −0.09 | 0.05 |
| 64 | $SPBr_3$ | 9.75 | 9.82 | 9.91 | 0.12 | 10.02 | −0.02 | 0.09 |
| 65 | $SeCl_2$ | 9.42 | 9.51 | 9.60 | 0.05 | 9.65 | 0.02 | −0.02 |
| 66 | $SeO_2$ | 11.96 | 11.98 | 12.02 | 0.09 | 12.11 | −0.01 | 0.19 |
| 67 | $SiBrF_3$ | 12.17 | 12.22 | 12.28 | 0.05 | 12.33 | −0.17 | 0.10 |
| 68 | $SiH_3I$ | 10.17 | 10.21 | 10.28 | 0.13 | 10.41 | −0.32 | 0.06 |
| 73 | $TiBr_4$ | 10.80 | 10.80 | 10.81 | 0.04 | 10.85 | −0.13 | 0.22 |
| 75 | $ZnBr_2$ | 11.02 | 11.04 | 11.06 | −0.03 | 11.04 | −0.17 | 0.14 |
| 79 | $ZrBr_4$ | 10.99 | 11.02 | 11.05 | −0.01 | 11.03 | −0.11 | 0.18 |
| 80 | $ZrCl_4$ | 11.98 | 12.07 | 12.18 | 0.11 | 12.30 | 0.01 | 0.19 |
| 81 | $ZrI_4$ | 9.69 | 9.73 | 9.81 | 0.22 | 10.03 | −0.29 | 0.14 |

# B QP energies for systems not included in the benchmark

Table 6: All $G_0W_0$@PBE QP energies calculated in this work for the systems which are not included in the benchmark: ADF results (TZ3P, QZ6P), BAND results (TZ3P+, QZ6P+), spin-orbit correction, and $G3W2$ correction, both calculated using ADF with the QZ6P basis set. All values are in eV.

| | | ADF | | BAND | | | |
|---|---|---|---|---|---|---|---|
| | Name | TZ3P | QZ6P | TZ3P+ | QZ6P+ | $\Delta_{\mathrm{SO}}$ | $\Delta_{G3W2}$ |
| 1 | AgBr | 8.76 | 8.85 | 9.05 | 9.03 | −0.10 | 0.10 |
| 2 | AgCl | 9.04 | 9.27 | 9.22 | 9.28 | −0.02 | 0.11 |
| 3 | AgI | 8.34 | 8.36 | 8.51 | 8.43 | −0.21 | 0.08 |
| 34 | CsCl | 7.75 | 7.66 | 7.54 | 7.77 | −0.02 | 0.07 |
| 35 | CsF | 7.93 | 8.03 | 7.90 | 8.33 | 0.00 | 0.19 |
| 36 | CsI | 6.81 | 6.78 | 6.92 | 6.80 | −0.16 | 0.07 |
| 37 | CuF | 9.45 | 9.57 | 9.76 | 9.44 | −0.03 | 0.18 |
| 44 | KI | 7.00 | 6.97 | 7.11 | 7.03 | −0.17 | 0.07 |
| 45 | $Kr_2$ | 12.87 | 13.03 | 13.18 | 13.14 | −0.09 | 0.11 |
| 46 | $KrF_2$ | 12.33 | 12.34 | 12.42 | 12.40 | −0.05 | 0.17 |
| 59 | RbBr | 7.29 | 7.26 | 7.44 | 7.51 | −0.02 | 0.08 |
| 60 | RbCl | 7.09 | 7.70 | 7.21 | 7.70 | −0.02 | 0.07 |
| 61 | RbI | 6.90 | 6.84 | 7.00 | 6.92 | −0.17 | 0.07 |
| 69 | $SrBr_2$ | 9.07 | 9.17 | 9.27 | 9.31 | −0.10 | 0.10 |
| 70 | $SrCl_2$ | 9.49 | 9.66 | 9.49 | 9.71 | −0.01 | 0.08 |
| 71 | $SrI_2$ | 8.49 | 8.51 | 8.59 | 8.64 | −0.19 | 0.08 |
| 72 | SrO | 5.51 | 6.20 | 5.51 | 6.02 | 0.00 | 0.04 |
| 74 | $TiI_4$ | 8.58 | 8.54 | 8.66 | 8.63 | −0.16 | 0.06 |
| 76 | $ZnCl_2$ | 10.81 | 11.00 | 10.82 | 10.92 | −0.03 | 0.10 |
| 77 | $ZnF_2$ | 12.58 | 12.47 | 12.58 | 12.38 | −0.01 | 0.24 |
| 78 | $ZnI_2$ | 9.23 | 9.22 | 9.33 | 9.36 | −0.21 | 0.07 |

Table 7: All ev$GW$@PBE0 QP energies calculated in this work for the systems which are not included in the benchmark: ADF results (TZ3P, QZ6P), BAND results (TZ3P+, QZ6P+), spin-orbit correction, and $G3W2$ correction, both calculated using ADF with the QZ6P basis set. All values are in eV.

| | | ADF | | BAND | | | |
|---|---|---|---|---|---|---|---|
| | Name | TZ3P | QZ6P | TZ3P+ | QZ6P+ | $\Delta_{\mathrm{SO}}$ | $\Delta_{G3W2}$ |
| 1 | AgBr | 9.01 | 9.13 | 9.22 | 9.17 | −0.12 | 0.14 |
| 2 | AgCl | 9.42 | 9.62 | 9.45 | 9.60 | −0.04 | 0.15 |
| 3 | AgI | 8.53 | 8.54 | 8.77 | 8.68 | −0.23 | 0.11 |
| 34 | CsCl | 7.88 | 8.10 | 7.92 | 8.15 | −0.03 | 0.11 |
| 35 | CsF | 8.63 | 8.80 | 8.58 | 8.99 | 0.00 | 0.25 |
| 36 | CsI | 7.08 | 7.12 | 7.20 | 7.08 | −0.22 | 0.08 |
| 37 | CuF | 9.33 | 9.64 | 9.57 | 9.76 | −0.01 | 0.31 |
| 44 | KI | 7.27 | 7.31 | 7.39 | 7.32 | −0.22 | 0.09 |
| 45 | $Kr_2$ | 13.09 | 13.29 | 13.62 | 13.44 | −0.11 | 0.12 |
| 46 | $KrF_2$ | 12.97 | 12.96 | 13.07 | 13.06 | −0.12 | 0.21 |
| 59 | RbBr | 7.60 | 7.71 | 7.83 | 7.84 | −0.11 | 0.10 |
| 60 | RbCl | 7.95 | 8.14 | 7.99 | 8.13 | −0.03 | 0.10 |
| 61 | RbI | 7.17 | 7.19 | 7.30 | 7.22 | −0.22 | 0.08 |
| 69 | $SrBr_2$ | 9.43 | 9.56 | 9.81 | 9.72 | −0.17 | 0.13 |
| 70 | $SrCl_2$ | 9.90 | 10.06 | 10.12 | 10.13 | −0.01 | 0.10 |
| 71 | $SrI_2$ | 8.80 | 8.83 | 9.07 | 8.94 | −0.23 | 0.10 |
| 72 | SrO | 5.72 | 5.95 | 5.90 | 6.01 | 0.00 | 0.19 |
| 74 | $TiI_4$ | 8.97 | 9.02 | 9.09 | 9.15 | −0.18 | 0.12 |
| 76 | $ZnCl_2$ | 11.20 | 11.38 | 11.21 | 11.34 | −0.03 | 0.12 |
| 77 | $ZnF_2$ | 13.19 | 13.11 | 13.22 | 13.10 | −0.02 | 0.30 |
| 78 | $ZnI_2$ | 9.52 | 9.56 | 9.67 | 9.71 | −0.26 | 0.08 |

Table 8: All $G_0W_0$@BHLYP QP energies calculated in this work for the systems which are not included in the benchmark: ADF results (TZ3P, QZ6P), BAND results (TZ3P+, QZ6P+), spin-orbit correction, and $G3W2$ correction, both calculated using ADF with the QZ6P basis set. All values are in eV.

| | Name | ADF | | BAND | | $\Delta_{\mathrm{SO}}$ | $\Delta_{G3W2}$ |
|---|---|---|---|---|---|---|---|
| | | TZ3P | QZ6P | TZ3P+ | QZ6P+ | | |
| 1 | AgBr | 9.16 | 9.29 | 9.37 | 9.39 | −0.14 | 0.16 |
| 2 | AgCl | 9.63 | 9.78 | 9.64 | 9.80 | −0.04 | 0.17 |
| 3 | AgI | 8.66 | 8.69 | 8.77 | 8.81 | −0.26 | 0.13 |
| 34 | CsCl | 8.12 | 8.35 | 8.13 | 8.41 | −0.04 | 0.13 |
| 35 | CsF | 9.00 | 9.21 | 8.90 | 9.28 | 0.00 | 0.28 |
| 36 | CsI | 7.25 | 7.29 | 7.37 | 7.27 | −0.25 | 0.10 |
| 37 | CuF | 9.71 | 9.92 | 9.82 | 9.77 | −0.02 | 0.36 |
| 44 | KI | 7.45 | 7.49 | 7.57 | 7.53 | −0.25 | 0.10 |
| 45 | $Kr_2$ | 13.28 | 13.47 | 13.66 | 13.64 | −0.12 | 0.12 |
| 46 | $KrF_2$ | 13.45 | 13.58 | 13.48 | 13.60 | −0.12 | 0.26 |
| 59 | RbBr | 7.78 | 7.91 | 8.00 | 8.02 | −0.13 | 0.12 |
| 60 | RbCl | 8.18 | 8.39 | 8.20 | 8.38 | −0.03 | 0.13 |
| 61 | RbI | 7.34 | 7.37 | 7.47 | 7.40 | −0.25 | 0.10 |
| 69 | $SrBr_2$ | 9.65 | 9.79 | 10.00 | 9.95 | −0.14 | 0.15 |
| 70 | $SrCl_2$ | 10.15 | 10.34 | 10.34 | 10.42 | −0.01 | 0.12 |
| 71 | $SrI_2$ | 9.01 | 9.05 | 9.27 | 9.17 | −0.27 | 0.12 |
| 72 | SrO | 5.91 | 6.07 | 5.10 | 5.97 | 0.00 | 0.29 |
| 73 | $TiBr_4$ | 10.46 | 10.63 | 10.69 | 10.77 | −0.10 | 0.22 |
| 76 | $ZnCl_2$ | 11.46 | 11.64 | 11.47 | 11.63 | −0.04 | 0.14 |
| 77 | $ZnF_2$ | 13.50 | 13.59 | 13.50 | 13.59 | −0.02 | 0.35 |
| 78 | $ZnI_2$ | 9.76 | 9.81 | 9.91 | 9.95 | −0.29 | 0.10 |

Table 9: All ev$GW$@PBE0 QP energies calculated in this work for the systems which are not included in the benchmark: ADF results (TZ3P, QZ6P), BAND results (TZ3P+, QZ6P+), spin-orbit correction, and $G3W2$ correction, both calculated using ADF with the QZ6P basis set. All values are in eV.

| | Name | ADF | | BAND | | | |
|---|---|---|---|---|---|---|---|
| | | TZ3P | QZ6P | TZ3P+ | QZ6P+ | $\Delta_{\mathrm{SO}}$ | $\Delta_{G3W2}$ |
| 1 | AgBr | 9.41 | 9.58 | 9.67 | 9.74 | −0.11 | 0.18 |
| 2 | AgCl | 9.93 | 10.11 | 9.95 | 10.13 | −0.04 | 0.20 |
| 3 | AgI | 8.85 | 8.83 | 9.00 | 8.99 | −0.20 | 0.14 |
| 34 | CsCl | 8.37 | 8.60 | 8.35 | 8.62 | −0.03 | 0.15 |
| 35 | CsF | 9.43 | 9.63 | 9.35 | 9.74 | 0.00 | 0.35 |
| 36 | CsI | 7.38 | 7.43 | 7.52 | 7.47 | −0.24 | 0.11 |
| 37 | CuF | 10.16 | 10.51 | 10.35 | 10.33 | 0.01 | 0.45 |
| 44 | KI | 7.57 | 7.63 | 7.72 | 7.65 | −0.25 | 0.11 |
| 45 | $Kr_2$ | 13.39 | 13.61 | 13.76 | 13.80 | −0.12 | 0.14 |
| 46 | $KrF_2$ | 13.62 | 13.78 | 13.72 | 13.85 | −0.09 | 0.30 |
| 59 | RbBr | 7.96 | 8.13 | 8.21 | 8.28 | −0.12 | 0.14 |
| 60 | RbCl | 8.41 | 8.64 | 8.41 | 8.65 | −0.03 | 0.15 |
| 61 | RbI | 7.47 | 7.52 | 7.61 | 7.60 | −0.25 | 0.11 |
| 69 | $SrBr_2$ | 9.78 | 9.95 | 10.18 | 10.09 | −0.13 | 0.16 |
| 70 | $SrCl_2$ | 10.28 | 10.49 | 10.50 | 10.51 | −0.01 | 0.14 |
| 71 | $SrI_2$ | 9.08 | 9.14 | 9.38 | 9.28 | −0.26 | 0.13 |
| 72 | SrO | 6.37 | 6.50 | 5.73 | 6.58 | 0.00 | 0.34 |
| 74 | $TiI_4$ | 9.31 | 9.36 | 9.49 | 9.51 | −0.22 | 0.17 |
| 76 | $ZnCl_2$ | 11.62 | 11.83 | 11.63 | 11.83 | −0.03 | 0.15 |
| 77 | $ZnF_2$ | 14.02 | 14.19 | 14.04 | 14.13 | −0.02 | 0.40 |
| 78 | $ZnI_2$ | 9.83 | 9.88 | 9.99 | 10.06 | −0.30 | 0.11 |

Table 10: qs$GW$ QP energies calculated in this work for the systems which are not included in the benchmark: ADF results (TZ3P, QZ6P), correction due to difference of ev$GW$ QP energies calculated with ADF and BAND, spin-orbit correction, and $G3W2$ correction (the latter two calculated using ADF with the QZ6P basis set). All values are in eV.

| | | ADF | | | | |
|---|---|---|---|---|---|---|
| Index | Name | TZ3P | QZ6P | $\Delta_{evGW}$ | $\Delta_{\mathrm{SO}}$ | $\Delta_{G3W2}$ |
| 1 | AgBr | 9.56 | 9.59 | 0.04 | −0.16 | 0.18 |
| 2 | AgCl | 10.00 | 10.10 | 0.08 | −0.05 | 0.19 |
| 3 | AgI | 8.93 | 8.96 | 0.17 | −0.29 | 0.14 |
| 34 | CsCl | 8.43 | 8.60 | 0.13 | −0.04 | 0.15 |
| 35 | CsF | 9.74 | 9.83 | 0.39 | 0.00 | 0.29 |
| 36 | CsI | 7.43 | 7.50 | −0.14 | −0.32 | 0.11 |
| 37 | CuF | 10.80 | 10.76 | −0.64 | −0.03 | 0.39 |
| 44 | KI | 7.62 | 7.69 | −0.18 | −0.32 | 0.11 |
| 45 | $Kr_2$ | 13.62 | 13.68 | −0.04 | −0.15 | 0.13 |
| 46 | $KrF_2$ | 13.93 | 13.94 | 0.06 | −0.08 | 0.27 |
| 59 | RbBr | 8.14 | 8.16 | 0.02 | −0.17 | 0.14 |
| 60 | RbCl | 8.48 | 8.64 | 0.00 | −0.05 | 0.14 |
| 61 | RbI | 7.53 | 7.58 | −0.01 | −0.32 | 0.11 |
| 69 | $SrBr_2$ | 10.00 | 10.03 | −0.17 | −0.17 | 0.16 |
| 70 | $SrCl_2$ | 10.42 | 10.57 | −0.23 | −0.04 | 0.13 |
| 71 | $SrI_2$ | 9.21 | 9.28 | −0.13 | −0.33 | 0.13 |
| 72 | SrO | 6.47 | 6.56 | 0.63 | 0.01 | 0.35 |
| 74 | $TiI_4$ | 9.44 | 9.45 | 0.10 | −0.29 | 0.17 |
| 76 | $ZnCl_2$ | 11.75 | 11.86 | 0.07 | −0.04 | 0.15 |
| 77 | $ZnF_2$ | 14.21 | 14.17 | −0.14 | −0.02 | 0.38 |
| 78 | $ZnI_2$ | 9.97 | 10.02 | 0.20 | −0.31 | 0.10 |

## C Basis sets for BAND calculations

The basis set files used for the BAND calculations are TZ3P and QZ6P basis sets,[1] augmented with additional high-angular-momentum functions. The basis set files are provided as .txt files which list all exponents for each angular momentum.

## References

(1) Förster, A.; Visscher, L. GW100: A Slater-Type Orbital Perspective. *J. Chem. Theory Comput.* **2021**, *17*, 5080–5097.
